# Supplementary material for: Complexity and Avoidance
Source: arXiv:2204.11289 source file (2022-04-24)
Supplement: Supplementary file 1 [file Appendix.tex]

\section{Existence of a Universal Prefix-Free Machine}

\begin{notation}
Let $\#_h$ denote the bijection $\#_h \colon h^\ast \to \mathbb{N}$ defined by ordering $h^\ast$ with respect to the shortlex order (as in the case of $\{0,1\}^\ast$, the shortlex order defines a well-ordering of $h^\ast$ of order type $\omega$). 
\end{notation}

\begin{prop} \label{universal prefix-free machine exists}
There exists a universal prefix-free machine $U \colonsub \{0,1\}^\ast \to h^\ast$.
\end{prop}
\begin{proof}
The standard proofs (e.g., \cite[Theorem 6.2.3]{simpson2007computability}) that there is a universal prefix-free machine $U \colonsub \{0,1\}^\ast \to \{0,1\}^\ast$ goes through with minor adjustments. For completeness, we recreate the proof given in \cite[Theorem 6.2.3]{simpson2007computability}:

Fix an admissible enumeration of the one-place partial recursive functions $\varphi_0,\varphi_1,\varphi_2,\ldots$. By $\varphi_{e,s}$ we mean the partial recursive function which on input $x$ computes $\varphi_e(x)$ for at most $s$-many steps (with respect to some model of computation), outputting $\varphi_e(x)$ if it has converged in $s$ steps, and undefined otherwise.

For each $e \in \mathbb{N}$, define $M_e \colonsub \{0,1\}^\ast \to h^\ast$ by
\begin{equation*}
M_e(\tau) \simeq \sigma \quad \text{if and only if} \quad \varphi_e(\#_2(\tau)) \simeq \#_h(\sigma).
\end{equation*}
$M_0,M_1,M_2,\ldots$ is an enumeration of all partial recursive functions ${\subseteq} \{0,1\}^\ast \to h^\ast$. In general $M_e$ is not necessarily prefix-free, so to correct for this we define machines $M_{e,s} \colonsub \{0,1\}^\ast \to h^\ast$ for each $s \in \mathbb{N}$ by
\begin{equation*}
M_{e,s}(\tau) \simeq \sigma \quad \text{if and only if} \quad \bigl(\#_2(\tau) < s\bigr) \wedge \bigl(\varphi_{e,s}(\#_2(\tau)) \simeq \#_h(\sigma)\bigr).
\end{equation*}
Some observations:
\begin{enumerate}[(i)]
\item The predicates $R(e,s,\tau) \equiv M_{e,s}(\tau) \converge$ and $S(e,s,\tau,\sigma) \equiv M_{e,s}(\tau) \simeq \sigma$ are recursive.
\item If $M_{e,s}(\tau) \simeq \sigma$, then $M_{e,t}(\tau) \simeq \sigma$ for all $t \geq s$.
\item $M_e(\tau) \simeq \sigma$ if and only if there is an $s \in \mathbb{N}$ such that $M_{e,s}(\tau) \simeq \sigma$.
\end{enumerate}

Now define $\tilde{M}_e$ by
\begin{equation*}
\tilde{M}_e(\tau) \simeq \sigma \quad \text{if and only if} \quad \exists s ~ ( M_{e,s}(\tau) \simeq \sigma \wedge \text{$\dom(M_{e,s})$ is prefix-free}).
\end{equation*}
Observation (i) implies $\tilde{M}_e$ is partial recursive, (ii) implies $\dom \tilde{M}_e$ is prefix-free, and (iii) implies $\tilde{M}_e = M_e$ if $\dom M_e$ is prefix-free. Observation (i) in fact implies that $\tilde{M}_e(\tau)$ is partial recursive as a function of both $e$ and $\tau$. It follows that $\tilde{M}_0,\tilde{M}_1,\tilde{M}_2,\ldots$ is an effective enumeration of the prefix-free machines. 

Finally, define $U$ by
\begin{equation*}
U( \langle\underbrace{0,\ldots,0}_{\text{$e$-many}},1\rangle \concat \tau) \simeq \tilde{M}_e(\tau).
\end{equation*}
$U$ is a universal prefix-free machine, as desired.
\end{proof}

\section{Existence of a Universal Left r.e. Continuous Semimeasure}

We wish to show that there is a universal left r.e. continuous semimeasure. One way to do this is to define -- in a fashion analogous to the argument in the proof of \cref{existence of universal prefix-free machine} -- a universal monotone machine, and subsequently show that a universal monotone machine gives rise to a universal left r.e. continuous semimeasure.

\begin{thm} \label{levin and zvonkin} (Levin, Zvonkin)
\begin{enumerate}[(a)]
\item For every monotone machine $M$, the function $\nu_M(\sigma) = \lambda(\{ X \in h^\mathbb{N} \mid M(X) \supseteq \sigma\})$ is a left r.e. continuous semimeasure.
\item For every left r.e. continuous semimeasure $\nu$ on $h^\mathbb{N}$, there is a monotone machine $M$ such that $\nu = \nu_M$.
\end{enumerate}
\end{thm}
\begin{proof} ~
\begin{enumerate}[(a)]
\item Suppose $M$ is a monotone machine. Because $\lambda$ is a probability measure on $\cantor$, $\nu_M(\langle\rangle) \leq 1$. Now suppose $\sigma \in h^\ast$. Then
\begin{align*}
\nu_M(\sigma) & = \lambda(\bbracket{M^{-1}(\sigma)}) \\
& = \lambda\left( \bigcup_{i < h(|\sigma|)}{\bbracket{M^{-1}(\sigma\concat \langle i\rangle)}} \cup \{ X \mid M^X = \sigma\}\right) \\
& \geq \lambda\left( \bigcup_{i < h(|\sigma|)}{\bbracket{M^{-1}(\sigma\concat \langle i \rangle)}}\right) \\
& = \sum_{i < h(|\sigma|)}{\lambda(\bbracket{M^{-1}(\sigma\concat \langle i \rangle)})} \\
& = \sum_{i < h(|\sigma|)}{\nu_M(\sigma)}.
\end{align*}
Thus, $\nu_M$ is a continuous semimeasure. The uniform monotone approximations 
\begin{equation*}
\nu_M(\sigma,s) \coloneq \lambda(\bbracket{\{\tau \in \{0,1\}^{\leq s} \mid M_s^\tau \converge \supseteq \sigma\}})
\end{equation*}
show that $\nu_M$ is left r.e.

\item Suppose $\nu$ is a left r.e. continuous semimeasure on $h^\mathbb{N}$. Assume without loss of generality that the uniform monotone approximations $\nu(\sigma,s)$ satisfy the following properties for each $s \in \mathbb{N}$:
\begin{enumerate}[(i)]
\item $\nu(\sigma,s)$ is a dyadic rational for every $\sigma \in h^\mathbb{N}$. 
\item If $|\sigma| \geq s$, then $\nu(\sigma,s) = 0$.
\item There is at most one $\sigma$ such that $\nu(\sigma,s) \neq \nu(\sigma,s+1)$.
\item If $\nu(\sigma,s) \neq \nu(\sigma,s+1)$, then $\nu(\sigma,s+1) = \nu(\sigma,s) + \frac{n}{2^{s+1}}$ for some $n \in \mathbb{N}$.
\item For all $\sigma$, $\nu(\sigma,s) \geq \sum_{i < h(|\sigma|)}{\nu(\sigma \concat \langle i \rangle, s)}$.
\end{enumerate}

To define $M$, we define a recursive sequence of partial approximations to $M$,
\begin{equation*}
\emptyset = M_0 \subseteq M_1 \subseteq M_2 \subseteq \cdots \subseteq M_s \subseteq M_{s+1} \subseteq \cdots
\end{equation*}
and let $M = \bigcup_{s \in \mathbb{N}}{M_s}$. For each $s$, we ensure that the following holds for all $\sigma \in h^\ast$ and $s \in \mathbb{N}$:
\begin{enumerate}[(I)]
\item $M_s$ is a monotone machine.
\item The set $D_s(\sigma) \coloneq \{ \tau \in \{0,1\}^\ast \mid (\tau,\sigma) \in M_s\}$ is prefix-free.
\item $\lambda(\bbracket{D_s(\sigma)}) = \nu(\sigma,s)$.
\item If $|\tau| > s$, then $\tau \notin D_s(\sigma)$.
\item If $\sigma \subseteq \sigma'$, then $\bbracket{D_s(\sigma')} \subseteq \bbracket{D_s(\sigma)}$.
\end{enumerate}
$M_0 \coloneq \emptyset$ clearly satisfies the above conditions, so suppose $M_s$ does as well. If $\nu(\sigma,s) = \nu(\sigma,s+1)$ for all $\sigma \in h^{< s}$, then let $M_{s+1} = M_s$. Otherwise, let $\sigma$ be the unique string such that $\nu(\sigma,s) \neq \nu(\sigma,s+1)$. By hypothesis, there is $n \in \mathbb{N}$ such that $\nu(\sigma,s+1) = \nu(\sigma,s) + \frac{n}{2^{s+1}}$. 

To define $M_{s+1}$, we make use of the following lemma.

\begin{lem} \label{levin-zvonkin proof lemma}
If $S,T \subseteq h^{\leq s}$ then there exists $R \subseteq h^s$ such that $\bbracket{R} = \bbracket{S} \setminus \bbracket{T}$.
\end{lem}
\begin{proof}
Define $R$ by
\begin{equation*}
R \coloneq \{ \sigma \in h^s \mid \bbracket{\sigma} \subseteq \bbracket{S} \wedge \bbracket{\sigma} \cap \bbracket{T} = \emptyset\}.
\end{equation*}
By construction, $\bbracket{R} \subseteq \bbracket{S}$ and $\bbracket{R} \cap \bbracket{T} = \emptyset$, so $\bbracket{R} \subseteq \bbracket{S} \setminus \bbracket{T}$. Conversely, given $X \in \bbracket{S} \setminus \bbracket{T}$, then $\bbracket{X \restrict s} \subseteq \bbracket{S}$. Because no element of $T$ extends to $X$ and all members of $T$ have length at most $s$ it follows that every member of $T$ is incompatible with $X \restrict s$, i.e., $\bbracket{X \restrict s} \cap \bbracket{T} = \emptyset$. Thus $X \restrict s \in R$ and hence $X \in \bbracket{R}$, showing $\bbracket{R} \supseteq \bbracket{S} \setminus \bbracket{T}$.
\end{proof}

We also observe that in \cref{levin-zvonkin proof lemma} the set $R$ can be determined uniformly and effectively from $S$ and $T$. 

We consider two cases, depending on whether $\sigma = \langle\rangle$ or not.
\begin{description}
\item[Case 1: $\sigma = \langle\rangle$.] By \cref{levin-zvonkin proof lemma} there is $R \subseteq h^{s+1}$ such that $\bbracket{R} = \bbracket{\langle\rangle} \setminus \bbracket{D_s(\langle\rangle)}$. Let $T_s$ be the first $n$ elements of $R$ ordered lexicographically. 

\item[Case 2: $\sigma \neq \langle\rangle$.] Let $\sigma_- = \sigma \restrict (|\sigma|-1)$ and $j = \sigma(|\sigma|-1)$ (so that $\sigma_- \concat \langle j \rangle = \sigma$). By \cref{levin-zvonkin proof lemma} there is $R \subseteq h^{s+1}$ such that 
\begin{equation*}
\bbracket{R} = \bbracket{D_s(\sigma_-)} \setminus \bbracket{D_s(\sigma_- \concat \langle 0 \rangle) \cup D_s(\sigma_- \concat \langle 1 \rangle) \cup \cdots \cup D_s(\sigma_- \concat \langle h(|\sigma|-1)-1 \rangle)}.
\end{equation*}
By hypothesis, for each $i < h(|\sigma|-1)$, $D_s(\sigma_- \concat \langle i \rangle) \subseteq D_s(\sigma)$, so
\begin{align*}
\lambda(\bbracket{R}) & = \lambda(\bbracket{D_s(\sigma_-)}) - \sum_{i < h(|\sigma|-1)}{D_s(\sigma_- \concat \langle i \rangle)} \\
& = \nu(\sigma_-,s) - \sum_{i < h(|\sigma|-1)}{\nu(\sigma_- \concat \langle i \rangle,s)} \\
& = \nu(\sigma_-,s+1) - \sum_{i < h(|\sigma|-1)}{\nu(\sigma_- \concat \langle i \rangle,s+1)} + \frac{n}{2^{s+1}} \\
& \geq \frac{n}{2^{s+1}}.
\end{align*}
It follows that $R$ contains at least $n$ elements, so let $T_s$ consist of the first $n$ elements of $R$ ordered lexicographically.
\end{description}

Finally, we let $M_{s+1} = M_s \cup \{ \langle\tau,\sigma\rangle \mid \tau \in T_s\}$. We must show that $M_{s+1}$ satisfies the necessary conditions to finish the construction of $M$. 

\begin{description}
\item[Claim 1.] $M_{s+1}$ is a monotone machine.

\begin{proof}
Because $M_s$ is a monotone Turing functional by hypothesis, it suffices to show that whenever $\langle\pi,\rho\rangle$ is a member of $M_s$ and $\tau$ is a member of $T_s$ extending $\pi$, then $\rho \subseteq \sigma$. The other direction -- namely that whenever $\pi$, $\rho$, and $\tau$ are such that $\langle\pi,\rho\rangle \in M_s$, $\tau \in T_s$, and $\tau \subseteq \pi$ then $\sigma \subseteq \rho$ -- holds vacuously as our hypotheses on $M_s$ show that $|\pi| \leq s$ and $|\tau| = s+1$. So suppose $\langle\pi,\rho\rangle \in M_s$ and $\pi \subseteq \tau \in T_s$. The definition of $T_s \subseteq R$ implies $\tau$ has an initial segment $\tau'$ such that $\langle\tau',\sigma_-\rangle \in M_s$ as $\bbracket{\tau} \subseteq \bbracket{R} \subseteq \bbracket{D_s(\sigma_-)}$. The monotonicity of $M_s$ implies that $\tau'$ and $\pi$ are compatible, as are $\sigma_-$ and $\rho$. If $\rho \subseteq \sigma_-$, then we are done. Otherwise, $\rho \supseteq \sigma_- \concat \langle k \rangle$ for some $k < h(|\sigma|-1)$, but this implies $\bbracket{\pi} \subseteq \bigcup_{i < h(|\sigma|-1)}{\bbracket{D_s(\sigma_- \concat \langle i \rangle)}}$ and hence $\bbracket{\tau} \subseteq \bigcup_{i < h(|\sigma|-1)}{\bbracket{D_s(\sigma_- \concat \langle i \rangle)}}$, yielding a contradiction. 
\end{proof}

\item[Claim 2.] $D_{s+1}(\sigma) = D_s(\sigma) \cup T_s$ and if $\sigma' \neq \sigma$, then $D_{s+1}(\sigma') = D_s(\sigma')$.

\begin{proof}
By construction.
\end{proof}

\item[Claim 3.] $D_{s+1}(\sigma)$ is prefix-free. 

\begin{proof}
$D_s(\sigma)$ is prefix-free by hypothesis and $T_s$ is prefix-free because its members all have equal length. To show that $D_{s+1}(\sigma) = D_s(\sigma) \cup T_s$, it suffices to show that elements of $D_s(\sigma)$ and $T_s$ are pairwise incompatible. Suppose $\tau \in D_s(\sigma)$ and $\pi \in T_s$. Because $\tau \in D_s(\sigma)$ it follows that $\bbracket{\tau} \subseteq \bigcup_{i < h(|\sigma|-1)}{\bbracket{D_s(\sigma_-\concat \langle i \rangle)}}$ and hence $\bbracket{\tau} \cap \bbracket{R} = \emptyset$. Because $\pi \in T_s \subseteq R$, we additionally have $\bbracket{\tau} \cap \bbracket{\pi} = \emptyset$, i.e., $\tau$ and $\pi$ are incompatible.
\end{proof}

\end{description}

The remaining conditions all follow from the construction. E.g., 
\begin{align*}
\lambda(\bbracket{D_{s+1}(\sigma)}) & = \lambda(\bbracket{D_s(\sigma)} \cup \bbracket{T_s}) \\
& = \lambda(\bbracket{D_s(\sigma)}) + \lambda(\bbracket{T_s}) \\
& = \nu(\sigma,s) + n2^{s+1} \\
& = \nu(\sigma,s+1).
\end{align*}

Because $M_s$ is a monotone machine for each $s$ and the sequence $\langle M_s \rangle_{s \in \mathbb{N}}$ is recursive, $M \coloneq \bigcup_{s \in \mathbb{N}}{M_s}$ is a monotone machine as well. 

It remains to show that $M$ has the desired property, i.e., $\nu = \nu_M$. Given $\sigma \in h^\ast$, 
\begin{align*}
\nu_M(\sigma) & = \lambda(\bbracket{M^{-1}(\sigma)}) \\
& = \lambda\left( \bigcup_{s \in \mathbb{N}}{\bbracket{M_s^{-1}(\sigma)}}\right) \\
& = \lim_{s \to \infty}{\lambda(\bbracket{M_s^{-1}(\sigma)})} \\
& = \lim_{s \to \infty}{\nu_{M_s}(\sigma)} \\
& = \lim_{s \to \infty}{\nu(\sigma,s)} \\
& = \nu(\sigma).
\end{align*}
\end{enumerate}
\end{proof}

\begin{lem}
There exists a \textdef{universal} monotone machine, i.e., a monotone machine $U$ such that for any other monotone machine $M$ there exists a string $\rho \in \{0,1\}^\ast$ such that $U(\rho\concat \sigma) \simeq M(\sigma)$ for all $\sigma \in \{0,1\}^\ast$. 
\end{lem}
\begin{proof}
By replacing the definition of $\tilde{M}_e$ with 
\begin{equation*}
\tilde{M}_e(\tau) \simeq \sigma \quad \text{if and only if} \quad \exists s ~ ( M_{e,s}(\tau) \simeq \sigma \wedge \text{$M_{e,s}$ is monotone})
\end{equation*}
and observing that $\tilde{M}_e$ is a monotonic machine and $\tilde{M}_e = M_e$ if and only if $M_e$ is a monotone machine, the proof of \cref{universal prefix-free machine exists} goes through to show that a universal monotone machine exists.
\end{proof}

\begin{prop}
There exists a universal left r.e. semimeasure $\mathbf{M}$ on $h^\ast$.
\end{prop}
\begin{proof}
It suffices to show that if $U$ is a universal monotone machine then $\mathbf{M} \coloneq \nu_U$ (as defined in \cref{levin and zvonkin}) is a universal left r.e. continuous semimeasure. If $\rho$ is another left r.e. continuous semimeasure, then \cref{levin and zvonkin} shows there is a monotone machine $M$ such that $\nu = \nu_M$. The universality of $U$ implies there is a $\rho \in \{0,1\}^\ast$ such that $U(\rho \concat \tau) \simeq M(\tau)$ for all $\tau \in \{0,1\}^\ast$. Then for $\sigma \in h^\ast$,
\begin{align*}
\nu(\sigma) & = \lambda(\bbracket{M^{-1}(\sigma)}) \\
& = \lambda(\{ X \in \cantor \mid M^X \supseteq \sigma \}) \\
& = \lambda(\{ X \in \cantor \mid \exists n ~ (M(X \restrict n) \supseteq \sigma)\}) \\
& = \lambda(\{ X \in \cantor \mid \exists n ~ (U( \rho \concat (X \restrict n)) \supseteq \sigma)\}) \\
& = 2^{|\rho|} \cdot \lambda(\bbracket{U^{-1}(\sigma)} \cap \bbracket{\rho}) \\
& \leq 2^{|\rho|} \lambda(\bbracket{U^{-1}(\sigma)}) \\
& = 2^{|\rho|} \mathbf{M}(\sigma).
\end{align*}
\end{proof}

\section{Prefix-free Complexity Alternative Form}

\begin{lem}
If $U$ and $V$ are universal prefix-free machines, then there exists $c \in \mathbb{N}$ such that $|\pfc_U(\sigma) - \pfc_V(\sigma)| \leq \log_{\gamma(\sigma)}(1/2) \cdot c$ for all $\sigma \in h^\ast$.
\end{lem}
\begin{proof}
For any $\sigma \in h^\ast$, $\mu(\sigma) \leq \frac{1}{2^{|\sigma|}}$ since $2 \leq h(n)$ for all $n \in \mathbb{N}$. This implies $\gamma(\sigma) \leq \frac{1}{2}$ and hence $0 < \log_{\gamma(\sigma)}(1/2) \leq 1$ for all $\sigma \in h^\ast$. 

By the universality of $V$, there exists a $\rho \in \{0,1\}^\ast$ such that $V(\rho \concat \tau) \simeq U(\tau)$ for all $\tau \in \{0,1\}^\ast$. If $\sigma^\ast \in \dom U$ is such that $U(\sigma^\ast) = \sigma$ and $\pfc_U(\sigma) = \log_{\gamma(\sigma)}(1/2) \cdot |\sigma^\ast|$, then $V(\rho \concat \sigma^\ast) = U(\sigma^\ast) = \sigma$. It follows that
\begin{align*}
\pfc_V(\sigma) & \leq \log_{\gamma(\sigma)}(1/2) \cdot |\rho \concat \sigma^\ast| \\
& \leq \log_{\gamma(\sigma)}(1/2) \cdot (|\rho| + |\sigma^\ast|) \\
& = \pfc_U(\sigma) + \log_{\gamma(\sigma)}(1/2)\cdot |\rho|.
\end{align*}

Likewise, if $\rho' \in \{0,1\}^\ast$ is such that $U(\rho' \concat \tau) \simeq V(\tau)$ for all $\tau \in \{0,1\}^\ast$, then $\pfc_U(\sigma) \leq \pfc_V(\sigma) + |\rho'|$, so with $c = \max\{|\rho|,|\rho'|\}$ we have
\begin{equation*}
|\pfc_U(\sigma) - \pfc_V(\sigma)| \leq \log_{\gamma(\sigma)}(1/2) \cdot c
\end{equation*}
for all $\sigma \in h^\ast$.
\end{proof}

The role of the factor $\log_{\gamma(\sigma)}(1/2)$ in the definition of $\pfc$ is so that an analog of Kraft's Inequality holds in $h^\ast$:

\begin{prop} \label{kraft's inequality}
$\sum_{\sigma \in h^\ast}{\gamma(\sigma)^{\pfc(\sigma)}} \leq 1$.
\end{prop}
\begin{proof}
To each $\sigma \in h^\ast$ there is a (not necessarily unique) $\sigma^\ast \in \dom U$ such that $U(\sigma^\ast) = \sigma$ and $\pwt(\sigma) = \log_{\gamma(\sigma)}(1/2) \cdot |\sigma^\ast|$. Then
\begin{equation*}
\gamma(\sigma)^{\pfc(\sigma)} = \gamma(\sigma)^{\log_{\gamma(\sigma)}(1/2) \cdot |\sigma^\ast|} = 2^{-|\sigma^\ast|}.
\end{equation*}
Because $\dom U$ is prefix-free, it follows that $\sum_{\tau \in \dom U}{2^{-|\tau|}} \leq 1$, so 
\begin{equation*}
\sum_{\sigma \in h^\ast}{\gamma(\sigma)^{\pfc(\sigma)}} \leq \sum_{\tau \in \dom U}{2^{-|\tau|}} \leq 1.
\end{equation*}
\end{proof}

%\begin{cor}[Kraft's Inequality]
%In $\{0,1\}^\ast$, $\sum_{\sigma \in \{0,1\}^\ast}{2^{-\pfc(\sigma)}} \leq 1$.
%\end{cor}

\begin{definition}[$f$-complexity]
$X \in h^\mathbb{N}$ is \textdef{$f$-complex} if there exists $c \in \mathbb{N}$ such that $\pfc(X \restrict n) \geq f(X \restrict n) - \log_{\gamma(\sigma)}(1/2) \cdot c$ for all $n \in \mathbb{N}$.

In particular, when $h \equiv 2$, $X \in \cantor$ is $f$-complex if there is $c \in \mathbb{N}$ such that $\pfc(X \restrict n) \geq f(X \restrict n) - c$ for all $n \in \mathbb{N}$.
\end{definition}

\cite[Theorem 2.6]{higuchi2014propogation} shows that $f$-randomness and $f$-complexity in $\cantor$ are equivalent. By adapting their proof we can show that this continues to hold within $h^\mathbb{N}$ as well.

\begin{lem} \label{kc theorem}
Suppose $\langle d_k, \sigma_k \rangle_{k \in \mathbb{N}}$ is a recursive sequence of pairs $\langle d_k, \sigma_k\rangle \in \mathbb{N} \times h^\ast$ such that $\sum_{k=0}^\infty{\gamma(\sigma_k)^{d_k}} \leq 1$. Then there is a recursive sequence $\langle \tau_k \rangle_{k \in \mathbb{N}}$ of binary strings such that $|\tau_k| = \lceil \log_{1/2}(\gamma(\sigma_k)) \cdot d_k\rceil$. 

Consequently, there exists $c \in \mathbb{N}$ such that $\pfc(\sigma_k) \leq d_k + \log_{\gamma(\sigma_k)}(1/2) \cdot c$ for all $k \in \mathbb{N}$.
\end{lem}
\begin{proof}
If $\sum_{k=0}^\infty{\gamma(\sigma_k)^{d_k}} \leq 1$, then 
\begin{equation*}
\sum_{k=0}^\infty{2^{-\lceil \log_{1/2}(\gamma(\sigma_k)) \cdot d_k \rceil}} \leq \sum_{k=0}^\infty{2^{-\log_{1/2}(\gamma(\sigma_k)) \cdot d_k}} = \sum_{k=0}^\infty{\gamma(\sigma_k)^{d_k}} \leq 1.
\end{equation*}
Let $e_k = \lceil \log_{1/2}(\gamma(\sigma)) \cdot d_k \rceil$. 

The proof of \cite[Theorem 3.6.1]{downey2010algorithmic} shows that there exists a recursive sequence $\langle \tau_k \rangle_{k \in \mathbb{N}}$ of pairwise-incompatible binary strings $\tau_k$ with $|\tau_k| = e_k$. 

To show the ``consequently'' statement holds, define $M \colonsub \{0,1\}^\ast \to h^\ast$ by setting $M(\tau_k) = \sigma_k$ for $k \in \mathbb{N}$ and $M(\tau) \diverge$ for all other $\tau$. Then $ M$ is a prefix-free machine, so there is $\rho \in \{0,1\}^\ast$ such that $U(\rho \concat \tau) \simeq M(\tau)$ for all $\tau \in \{0,1\}^\ast$. In particular, $U(\rho \concat \tau_k) = \sigma_k$ and 
\begin{equation*}
|\rho \concat \tau_k| = |\tau_k| + |\rho| = e_k + |\rho| = \lceil \log_{1/2}(\gamma(\sigma)) \cdot d_k \rceil + |\rho|.
\end{equation*}
Thus,
\begin{align*}
\pfc(\sigma_k) & \leq \log_{\gamma(\sigma_k)}(1/2) \cdot |\rho \concat \tau_k| \\
& = \log_{\gamma(\sigma_k)}(1/2) \cdot \lceil \log_{1/2}(\gamma(\sigma_k)) \cdot d_k \rceil + \log_{\gamma(\sigma_k)}(1/2) \cdot |\rho| \\
& \leq \log_{\gamma(\sigma_k)}(1/2) \cdot \log_{1/2}(\gamma(\sigma_k)) \cdot d_k + \log_{\gamma(\sigma_k)}(1/2) \cdot (|\rho|+1) \\
& = d_k + \log_{\gamma(\sigma_k)}(1/2) \cdot (|\rho|+1).
\end{align*}
\end{proof}

\begin{thm}
$f$-randomness in $h^\mathbb{N}$ is equivalent to $f$-complexity in $h^\mathbb{N}$.
%For all $X \in h^\mathbb{N}$, $X$ is $f$-random if and only if it is $f$-complex.
\end{thm}
\begin{proof}
For $i \in \mathbb{N}$, let $S_i = \{ \sigma \in h^\ast \mid \pfc(\sigma) < f(\sigma) - \log_{\gamma(\sigma)}(1/2) \cdot i\}$. We claim that $\langle S_i \rangle_{i \in \mathbb{N}}$ forms an $f$-ML test. Indeed, 
\begin{equation*}
\dwt_f(S_i) = \sum_{\sigma \in S_i}{\gamma(\sigma)^{f(\sigma)}} < \sum_{\sigma \in S_i}{\gamma(\sigma)^{\pfc(\sigma)+\log_{\gamma(\sigma)}(1/2) \cdot i}} = \sum_{\sigma \in S_i}{\gamma(\sigma)^{\pfc(\sigma)} \cdot 2^{-i}} \leq 2^{-i}.
\end{equation*}
where the final inequality follows from \cref{kraft's inequality}. If $X$ is $f$-random, then $\langle S_i \rangle_{i \in \mathbb{N}}$ does not cover $X$, meaning there is $i \in \mathbb{N}$ such that $\pfc(X \restrict n) \geq f(X \restrict n) - \log_{\gamma(X \restrict n)}(1/2) \cdot i$ for all $n \in \mathbb{N}$ and hence $f$-complex.

Conversely, suppose $X$ is not $f$-random, and let $\langle S_i \rangle_{i \in \mathbb{N}}$ be an $f$-ML test covering $X$. Then
\begin{equation*}
\sum_{i = 0}^\infty{\sum_{\sigma \in S_{2i}}{\gamma(\sigma)^{f(\sigma) - \log_{\gamma(\sigma)}(1/2)\cdot (i+1)}}} = \sum_{i = 0}^\infty{2^i\gamma(\sigma)^{f(\sigma)}} \leq \sum_{i=0}^\infty{2^{i+1} \cdot 2^{-2i}} = \sum_{i=0}^\infty{2^{-i-1}} = 1.
\end{equation*}
Suppose $g_i \colon \mathbb{N} \to S_{2i}$ is a recursive surjection for each $i \in \mathbb{N}$ and let $g \colon \mathbb{N} \to \bigcup_{i \in \mathbb{N}}{S_{2i}}$ be defined by $g(\pi^{(2)}(i,j)) \coloneq g_i(j)$. Write $\sigma_k = g(k)$ and $d_k = f(\sigma_k) - \log_{\gamma(\sigma_k)}(1/2) \cdot ((k)_0+1)$. Then \cref{kc theorem} implies there exists $c \in \mathbb{N}$ such that $\pfc(\sigma_k) \leq f(\sigma_k) - \log_{\gamma(\sigma_k)}(1/2) \cdot ((k)_0 + 1 - c)$ for all $k \in \mathbb{N}$. Because $\langle S_i \rangle_{i \in \mathbb{N}}$ covers $X$, $\langle S_{2i} \rangle_{i \in I}$ does as well. Thus, for every $i \in \mathbb{N}$, there exists $n \in \mathbb{N}$ such that $\pfc(X \restrict n) \leq f(X \restrict n) - \log_{\gamma(X \restrict n)}(1/2) \cdot (i + 1 - c)$, so $X$ is not $f$-complex.
\end{proof}

$f$-randomness and $f$-complexity in $h^\mathbb{N}$ can be defined in an alternative way that resembles more closely the definitions of $f$-randomness and $f$-complexity in $\cantor$ at the cost of modifying the meaning of $f$ in `$f$-randomness' and `$f$-complexity'. Temporarily define, for $\sigma \in h^\ast$ and $S \subseteq h^\ast$,
\begin{equation*}
\dwt'_f(S) \coloneq \sum_{\sigma \in S}{2^{-f(\sigma)}} \quad \text{and} \quad 
\pfc'(\sigma) \coloneq \min \{ |\tau| \mid U(\tau) \simeq \sigma\}.
\end{equation*}
In other words, $\dwt'_f$ and $\pfc'$ are the definitions of $\dwt_f$ and $\pfc$ as they are in $\{0,1\}^\ast$, except with expanded domains $\mathcal{P}(h^\ast)$ and $h^\ast$, respectively.

\begin{prop}
Suppose $f \colon h^\ast \to \mathbb{R}$ is computable and $g(\sigma) = \log_{1/2}(\gamma(\sigma)) \cdot f(\sigma)$. 
\begin{enumerate}[(a)]
\item $\dwt_f(S) = \dwt'_g(S)$ for all $S \subseteq h^\ast$. Consequently, $X \in h^\mathbb{N}$ is $f$-random if and only if there exists no uniformly r.e. sequence $\langle S_k \rangle_{k \in \mathbb{N}}$ such that $\dwt'_g(S_k) \leq 1/2^k$ for each $k \in \mathbb{N}$ and $X \in \bigcap_{k \in \mathbb{N}}{\bbracket{S_k}}$.

\item $\pfc(\sigma) = \log_{\gamma(\sigma)}(1/2) \cdot \pfc'(\sigma)$ for all $\sigma \in h^\ast$. Consequently, $X \in h^\mathbb{N}$ is $f$-complex if and only if there exists $c \in \mathbb{N}$ such that $\pfc'(X \restrict n) \geq g(X \restrict n) - c$ for all $n \in \mathbb{N}$.
\end{enumerate}
\end{prop}
\begin{proof} ~
\begin{enumerate}[(a)]
\item For every $\sigma \in h^\ast$, $\gamma(\sigma)^{f(\sigma)} = (1/2)^{\log_{1/2}(\gamma(\sigma)) \cdot f(\sigma)} = 2^{-g(\sigma)}$. 

\item Suppose $\sigma^\ast \in \{0,1\}^\ast$ is such that $U(\sigma^\ast) \simeq \sigma$ and $|\sigma^\ast| = \min\{ |\tau| \mid U(\tau) \simeq \sigma\}$. Then
\begin{equation*}
\pfc(\sigma) = \log_{\gamma(\sigma)}(1/2) \cdot |\sigma^\ast| = \log_{\gamma(\sigma)}(1/2) \cdot \pfc'(\sigma).
\end{equation*}
\end{enumerate}
\end{proof}

\section{A Priori Complexity Alternative Form}

\begin{definition}[A Priori Complexity]
Fix a universal left r.e. semimeasure $\mathbf{M}$. The \textdef{a priori complexity} of a string $\sigma \in h^\ast$ is defined by
\begin{equation*}
\apc(\sigma) = \apc_\mathbf{M}(\sigma) \coloneq \log_{\gamma(\sigma)} \mathbf{M}(\sigma).
\end{equation*}
\end{definition}

As with prefix-free complexity, if $\mathbf{N}$ were another universal left r.e. semimeasure, then $\apc_\mathbf{M}$ and $\apc_\mathbf{N}$ differ by at most a constant.

\begin{definition}[Strong $f$-Complexity]
$X \in h^\mathbb{N}$ is \textdef{strongly $f$-complex} if there exists a $c \in \mathbb{N}$ such that $\apc(X \restrict n) \geq f(X \restrict n) - \log_{\gamma(X \restrict n)}(1/2) \cdot c$ for all $n \in \mathbb{N}$.
\end{definition}

\begin{thm} \label{equivalent characterizations of strong f-randomness}
Suppose $X \in h^\mathbb{N}$. The following are equivalent.
\begin{enumerate}[(i)]
\item $X$ is strongly $f$-random.
\item $X$ is strongly $f$-complex.
\item $d_0$ does not $f$-succeed on $X$, where $d_0$ is the universal left r.e. supermartingale corresponding to $\mathbf{M}$ as in \cref{relationship between supermartingales and continuous semimeasures}.
\item No left r.e. supermartingale $f$-succeeds on $X$.
\end{enumerate}
\end{thm}
\begin{proof}
\begin{description}
\item[$(i) \iff (ii)$] Suppose $X$ is strongly $f$-random. Let $S_i = \{ \sigma \in h^\ast \mid \apc(\sigma) < f(\sigma) - \log_{\gamma(\sigma)}(1/2) \cdot i\}$. If $P \subseteq S_i$ is prefix-free, then
\begin{equation*}
\dwt_f(P) = \sum_{\sigma \in P}{\gamma(\sigma)^{f(\sigma)}} \leq \sum_{\sigma \in P}{\gamma(\sigma)^{\apc(\sigma) + \log_{\gamma(\sigma)}(1/2) \cdot i}} \leq \frac{1}{2^i} \sum_{\sigma \in P}{\mathbf{M}(\sigma)} \leq \frac{1}{2^i} \mathbf{M}(\langle\rangle) \leq \frac{1}{2^i}.
\end{equation*}
Thus, $\langle S_i \rangle_{i \in \mathbb{N}}$ forms a weak $f$-ML test. Because $X$ is strongly $f$-random, $X$ is not covered by $\langle S_i \rangle_{i \in \mathbb{N}}$ and so there is an $i \in \mathbb{N}$ such that $X \notin \bbracket{S_i}$, i.e., for every $n \in \mathbb{N}$ we have $\apc(X \restrict n) \geq f(X \restrict n) - \log_{\gamma(\sigma)}(1/2) \cdot i$, so $X$ is strongly $f$-complex.

If $X$ is not strongly $f$-random, then there is a weak $f$-ML test $\langle S_i \rangle_{i \in \mathbb{N}}$ which covers $X$. Uniformly in $i \in \mathbb{N}$, we let $\nu_i$ be defined by $\nu_i(\sigma) = \pwt_f(\{ \tau \in S_i \mid \tau \supseteq \sigma\})$. $\nu_i$ is a continuous semimeasure; using \cref{pwt inequalities} we have
\begin{align*}
\nu_i(\sigma) & = \pwt_f(\{ \tau \in S_i \mid \tau \supseteq \sigma\}) \\
& \geq \pwt_f(\{ \tau \in S_i \mid \tau \supset \sigma\}) \\
& = \pwt_f(\bigcup_{j < h(|\sigma|)}{\{ \tau \in S_i \mid \tau \supseteq \sigma\concat\langle j \rangle\}}) \\
& = \sum_{j < h(|\sigma|)}{\pwt_f(\{ \tau \in S_i \mid \tau \supseteq \sigma\concat\langle j\rangle\})} \\
& = \sum_{j < h(|\sigma|)}{\nu_i(\sigma \concat \langle j\rangle)}.
\end{align*}
That $\nu_i$ is left r.e. follows from the fact that $S_i$ is r.e.
Observe that for $\tau \in S_i$ we have $\dwt_f(\tau) \leq \nu_i(\tau)$. Because $\nu_i(\langle\rangle) = \pwt_f(S_i) \leq 2^{-i}$ for each $i$, the map $\overline{\nu} \colon h^\ast \to [0,1]$ defined by
\begin{equation*}
\overline{\nu}(\sigma) = \sum_{i=0}^\infty{2^i \nu_{2i}(\sigma)}
\end{equation*}
is a left r.e. semimeasure, and hence there is $c \in \mathbb{N}$ such that $\overline{\nu}(\sigma) < c \cdot \mathbf{M}(\sigma)$ for all $\sigma \in h^\ast$. Then for $\sigma \in S_{2i}$, we have
\begin{equation*}
2^i \cdot \gamma(\sigma)^{f(\sigma)} = 2^i \dwt_f(\sigma) \leq 2^i \nu_{2i}(\sigma) \leq \overline{\nu}(\sigma) < c \cdot \mathbf{M}(\sigma) = \gamma(\sigma)^{\apc(\sigma) + \log_{\gamma(\sigma)}(1/2) \cdot \log_{1/2}(c)}
\end{equation*}
and hence
\begin{equation*}
\apc(\sigma) + \log_{\gamma(\sigma)}(1/2) \cdot (i + \log_{1/2}(c)) < f(\sigma).
\end{equation*}
Being covered by $\langle S_i \rangle_{i \in \mathbb{N}}$ and hence $\langle S_{2i} \rangle_{i \in \mathbb{N}}$, $X$ is not strongly $f$-complex.

\item[$(ii) \iff (iii)$] Let $d_0$ be the universal left r.e. supermartingale corresponding to $\mathbf{M}$, as in \cref{relationship between supermartingales and continuous semimeasures}. Now observe that for any $X \in h^\mathbb{N}$ and $n \in \mathbb{N}$,
\begin{equation*}
d_0(X \restrict n) \cdot \mu(X \restrict n)^{1 - f(X \restrict n)/n} = \mathbf{M}(X \restrict n) \cdot \mu(X \restrict n)^{-1} \cdot \mu(X \restrict n)^{1-f(X \restrict n)/n} = \gamma(X\restrict n)^{\apc(X\restrict n) - f(X \restrict n)}.
\end{equation*}
Thus,
\begin{equation*}
\limsup_n{d_0(X \restrict n) \cdot \mu(X \restrict n)^{1-f(X \restrict n)/n}} = \infty \quad \text{if and only if} \quad \forall c \exists n ~ (\apc(X \restrict n) < f(X \restrict n) - \log_{\gamma(X \restrict n)}(1/2) \cdot c)
\end{equation*} 
In other words, $d_0$ $f$-succeeds on $X$ if and only if $X$ is not strongly $f$-complex.

\item[$(iii) \iff (iv)$] If no left r.e. supermartingale $f$-succeeds on $X$, then in particular $d_0$ does not $f$-succeed on $X$. Conversely, if $d_0$ does not $f$-succeed on $X$, then the universality of $d_0$ shows that no left r.e. supermartingale $f$-succeeds on $X$. 
\end{description}
\end{proof}

\section{Solovay Randomness}
